# Supplementary material for: Efficient Backdoor Removal Through Natural Gradient Fine-tuning
Source: arXiv:2306.17441 source file (2023-06-30)
Supplement: Supplementary file 1 [file appendix.tex]

\section{Appendix}\label{sec:app}
\subsection{Backdoor Formulation}
Here, $\hat{x}_i = (1-m)\odot x_i + m\odot \Delta$ is the triggered input with target label $y^{(t)}_i \neq y_i$ set by the adversary. Whereas $m \in \{0,1\}^d$ is a binary mask, $\Delta \in \mathbb{R}^d$ is the trigger distribution (!), and $\odot$ represents element-wise dot-product. Depending on the type of trigger, poison rate ($|\mathbb{D}'_{\mathsf{train}}|/|\mathbb{D}_{\mathsf{train}}|$) and label mapping ($y^{(t)}_i \rightarrow y_i$), one can formulate different type of backdoor attacks. In addition to above mentioned label poisoning attack, we also consider clean label attack that will be discussed in the supplementary.

$\hat{x}_i = (1-m)\odot x_i + m\odot \Delta$ is the triggered input with target label $y^{(t)}_i \neq y_i$ set by the adversary. Whereas $m \in \{0,1\}^D$ is a binary mask, $\Delta \in \mathbb{R}^D$ is the trigger distribution, and $\odot$ represents element-wise dot-product.

Notice that $||m||_1<< D$ should be small enough so that the modified input and actual input are visually indistinguishable(this line is not correct, what is l1 and also you are talking about adversarial attack not backdoor). However, if $||m||_1$ is too small, then the backdoored network, $f_{\theta}$ will be unstable as,
\begin{equation}
\begin{aligned}[b]
    f_{\theta} (\hat{x}_i) &= f_\theta ((1-m)\odot x_i + m\odot \Delta)\\
    &= f_{\theta} (x_i + m\odot(\Delta - x_i)) \\
    &\approx  f_{\theta} (x_i) + \{m\odot(\Delta - x_i)\}^T \cdot \nabla_{\theta} f_{\theta} ~~\text{(Applying Taylor theorem)}
\end{aligned} 
\label{eqn:backapprox}
\end{equation}
so, the distribution of inserted trigger $m\odot\Delta$ would be large enough to persuade the weight landscape to memorize it, generating a sharpness in the weight space. 

\subsection{Proof of Lemma~\ref{lemma1}.}
\textbf{Lemma~\ref{lemma1}.} \textit{Whenever a backdoor trigger inserted in a training sample $x_i$ with a target label $y^{(t)}_i \neq y_i$, and whenever the model has enough capacity to minimize training loss, backdoor will create bias (e.g., sharp-peaks in weight space) towards backdoor distribution in the model as,}
\begin{gather*}
    \sum_{(x_i,y_i) \in \mathbb{D}_{\mathsf{train}}} \mathbb{E}\left[||\mathbf{y} - f^*(\hat{\mathbf{x}})||_2^2\right] >0 ~ \text{and}~ \sum_{(x_i,y_i) \in \mathbb{D}_{\mathsf{train}}} \mathbb{E}\left[||\mathbf{y}^{(t)} - f_{\theta}(\hat{\mathbf{x}})||_2^2\right] = 0 \Rightarrow \textsc{Skewed~Model.}
\end{gather*}

\textbf{Motivation-1:} Inserting backdoor is a process of overfitting to both clean and triggered data. Which causes to model have high variance and low bias. However, the overfitting phenomenon in this particular case can be slightly different from the overfitting of benign over-parameterized model (need experimentation!, we show this through weight loss landscape visualization). In Trojan model, the effect of trigger memorization ???!   

\textit{Observation/Fact.} Data Augmentation has been used as the means of reducing generalization error on the unseen data. \cite{wu2020generalization} observed that label-invariant transformations can add new information to the training data. ********

The weight space of Backdoored model contains extreme values or sharp-peaks which help it memorize the backdoor triggers.We will validate it using \textbf{graphical illustration} as well as the referring existing works~\cite{guo2021aeva}.

\textit{Hypothesis.} The data distributions of regular training data and backdoor triggers differ significantly which forces the model's weight space to learn the footprints of both distributions.

\subsubsection{Terminologies} (Move to Appendix?)
\textbf{Clean Test Accuracy (CA):} Accuracy on clean test samples.

\textbf{Attack Success Rate (ASR):} Misclassification rate of poison test samples to the target label. Percentage of poison test samples that has been successfully misclassified to the target label.  

\textbf{Poison Test Accuracy (PA):} Percentage of posion test samples that are correctly classified to their ground truth labels. 

\textbf{Clean Generalization Gap (CG):} Differences in clean test accuracies of a backdoor model to a benign model.

\textbf{Robust Generalization Gap (RG):} Differences in poison test accuracies of a backdoor model to a benign model.

\textbf{All2All Attack:} Target labels of the poison data are uniformly distributed among all class labels.

\textbf{All2one Attack:} All of the poison data has the same target label.

\begin{itemize}
    \item We are also using a technique like neuron pruning but with a much simpler objective function. From Motivation-1, we can deduce the impact of backdoor attack on the parameter space of DNN. First, We analyze what type of data distribution backdoored DNN learns during training. at the time of backdooring, DNN has to learn a different data distribution than the clean training, weight space is subject to have an unusual shape with extreme values or peaks. We want to unlearn the backdoor by reversing this process of \emph{shape shifting}. 
    \begin{itemize}
        \item We hope to regularize the model by flattening the weight loss landscape. We observe that one does not need adversarial training/any complicated objective function to regularize the model. \NK{on the contrary, we claim that adversarial training harms the process of backdoor removal as our experimentation shows. We will explain this.} Instead, we opt to use traditional augmentation based regularization which removes the backdoor and keep the generalization performance at the same level. 
        \begin{itemize}
            \item \emph{Weak Augmentation:} Through theoritical and empirical evaluation, we show that traditional weak augmentation only helps increasing the performance on clean samples while under-performing in removing backdoor. The purpose of weak augmentation is to learn feature that are useful for clean generalization performance. During fine-tuning with weak augmentations, the model memorizes the validation samples and does not change the weight loss landscape that much(can be observed from training accuracy and loss landscape). As a result, the anomalies/extremas are still there after fine-tuning. Since backdoor model already have high clean accuracy and our main goal is to remove the backdoor, weak augmentation is not the suitable for our work.
            \item \emph{Strong Augmentation:} Instead, strong augmentations (Jittering, color, posterize, invert, cutmiz, augmax etc.) make the training more challenging in terms of memorizing the validation samples. Furthermore, applying strong augmentations shifts the data distribution from the original distribution (\NK{However, the aug. dist. may not replicate the trigger distribution. In summary, the augmented data dist. is different from both original and triggered data distribution. But it is important to focus on the part that it is different from triggered data distribution.}) DNN becomes busy learning the new aug. dist. and eventually forgets about the learned triggered data distribution (need to elaborate and verify by heatmap). \textcolor{red}{We could not see this in the loss landscape!!!! --> As a result, the peak and anomalies created by the triggered data is also gone (see landscape)}       
        \end{itemize}
    \end{itemize}
\end{itemize}
\begin{table}[ht]
    \centering
    \scalebox{0.85}{
    \begin{tabular}{c|cc|cc|cc|cc}
    \toprule
    Attacks & \multicolumn{2}{c|}{Badnet} & \multicolumn{2}{c|}{SIG} & \multicolumn{2}{c|}{Blend} & \multicolumn{2}{c|}{Trojan} \\
    \midrule
    Augmentation & ASR & ACC & ASR & ACC & ASR & ACC&ASR & ACC\\
    \midrule
    Posterize & 0.81 & 94.91 &1.41 &87.61 &100 &94.85&1.43 &87.62\\
    Rotate & 10.0&91.23 &1.91 &84.26  &62.05 &90.15 &1.91 &84.23\\
    Solarize & 1.13&90.0 &1.42 &85.23  &99.42 &99.10&1.47 &85.01\\
    Autocontrast &0.73 &94.15&1.11 &86.22 &100    &94.72 &1.15&86.24\\
    Equalize &0.67 &91.64&0.55 &85.24  &57.73 &93.74&0.55 &85.24\\
    Invert & 0.73&94.95 &1.21 & 87.68 &99.94 &90.24&1.24 & 87.64\\
    Color &0.91&94.94&1.23&87.52  &100 &94.81&1.22&87.54 \\
    Sharpness &0.92& 94.54& 1.23&87.56 &100 &94.72& 1.22&87.53 \\
    ShearX & 0.76&94.72 &1.21&87.45  &100 &94.5&1.56&86.92\\
    Contrast &0.62&94.83 &1.23 &87.64 &100& 94.53&1.23 &87.63\\
    Brightness &0.73&94.82&1.04& 87.43 &100&94.52&1.04 & 87.43 \\   
    ShearY &0.55&94.77&0.93&87.57 &100 &94.24&0.92 &87.52\\
    TranslateY &0.68&94.39&0.94 &86.38    &100 &93.34&0.92 &86.33\\
    TranslateX &1.78&93.45 &1.13&87.65 &100&93.54&1.11 &87.62\\
    \bottomrule
    \end{tabular}
    }
    \vspace{2mm}
    \caption{Backdoor attack removal using only one of the strong augmentations instead of the policy. Poison Rate is only 5\%}
    \label{tab:attack_reomval_1_aug}
\end{table}

\begin{table}[!htp]

\small
\centering
\caption{The attack success rate (ASR \%) and the clean accuracy (CA \%)  of 4 backdoor defense methods against 10 backdoor attacks including 6 classic backdoor attacks and 4 feature-space attacks. \emph{None} means the training data is completely clean.}
  \label{tab1}
\begin{tabular}{c|c|cc|cc|cc|cc|cc|cc}
\toprule
\multirow{2}{*}{Dataset} & \multirow{2}{*}{Method} & \multicolumn{2}{c|}{\begin{tabular}[c|]{@{}c@{}}No Defense\end{tabular}} & \multicolumn{2}{c|}{MCR} & \multicolumn{2}{c|}{NAD} & \multicolumn{2}{c|}{ANP} &\multicolumn{2}{c|}{ABL}&  \multicolumn{2}{c}{\textbf{Ours}}\\ \cline{3-14} 
 &  & ASR & ACC & ASR & ACC & ASR & ACC & ASR & ACC & ASR & ACC & ASR & ACC\\ \hline
\multirow{8}{*}{CIFAR-10} 
& \emph{None} & 0 & 95.76 & 0 & 90.68 & 0 & 92.34 & 0 & 94.98 & 0 & 93.87 & 0 & 95.10  \\ %\cline{2-12} 
& BadNets &  100 & 90.73 & 3.97 & 81.65 & 4.32 & 85.41 & 2.84 & 84.96  & 3.73 & 87.12 & 1.54 & 89.20 \\

 & Blend & 100 & 93.98 & 32.72 & 80.19 & 5.18 & 84.89 & 3.81 & 89.10  & 16.79 & 87.40 & 0.43 & 91.94 \\
  & Trojan-one & 100 & 88.33 & 20.45 & 79.63  & 17.21 &  83.16 & 5.53 & 84.89 &  4.01 & 86.52 & 2.89 & 87.10 \\
   & Trojan-all & 100 & 89.67 & 22.34 & 80.92  & 18.73 & 83.87 & 5.47 & 85.20  & 4.82 & 86.18 & 2.13 & 87.35 \\
    & SIG & 99.60 & 88.94 & 0.89  & 82.26  & 2.07 & 84.27 & 0.37 & 84.60 &  0.26 & 87.10 &  0.08 & 87.05 \\
 & Dynamic-one & 100 & 92.87 & 24.93 & 78.62 & 23.09 & 82.71 & 1.78 & 85.26 & 18.12 & 88.12 & 0.45 & 90.84 \\
 & Dynamic-all & 100 & 92.61 & 26.12 & 77.90 & 22.61 & 81.01 & 2.19 & 84.51  & 16.31 & 87.55 & 0.67& 90.19  \\
  & CLB & 100 & 92.61 & 26.12 & 77.90 & 22.61 & 81.01 & 2.19 & 84.51  & 16.31 & 87.55 & 0.67& 90.19\\  %\\ \cline{2-12} 
  & FC & 87.62 & 84.59 &  40.71 & 81.95 & 53.22 & 83.84 & 3.71 & 82.23 & 1.14 & 82.49 & 1.06 & 83.01 \\\cline{2-12} 
 & \multicolumn{1}{l}{Mean ASR Drop} & \multicolumn{1}{|l}{97.73} & \multicolumn{1}{l}{83.55} & \multicolumn{1}{|l}{75.07} & \multicolumn{1}{l}{80.62} & \multicolumn{1}{|l}{24.38} & \multicolumn{1}{l}{76.56}
 & \multicolumn{1}{|l}{20.40} & \multicolumn{1}{l}{80.37}  & \multicolumn{1}{|c}{\textbf{7.69}} & \multicolumn{1}{c}{\textbf{84.76}} \\ \midrule
\multirow{6}{*}{GTSRB} 
& \emph{None} & 0 & 97.87 & 0 & 95.49 &  0 & 95.18 &  0 & 96.12 & 0 & 96.41 & 0 & 96.70 \\ %\cline{2-12} 
& BadNets & 100 & 97.38 & 1.00 & 93.45 & 0.19 & 89.52 & 0.35 & 93.17 & 0.03 & 96.01 & 0.14 & 96.11 \\
& Blend & 100 & 95.92 & 6.83 & 92.91 & 8.10 & 89.37 & 4.41 & 93.02 & 24.59 & 93.14 & 3.38 & 93.19 \\
& Trojan-one & 99.50 & 96.27 & 2.76 & 92.98 & 0.37 & 90.02 & 0.81 & 92.74 & 0.36 & 94.95 & 0.21 & 95.18 \\
& Trojan-all & 99.71 & 96.08 & 3.25 & 92.18  & 0.98 & 90.27 & 1.16 & 92.51 & 0.91 & 94.01 & 0.27 & 94.87 \\
& SIG & 97.13 & 96.93 & 33.98 & 91.83 & 4.64 & 89.36 & 8.17 & 91.82  & 5.13 & 96.33 & 3.24 & 95.48 \\
& Dynamic-one & 100 & 97.27 & 64.82 & 43.91 & 68.71 & 76.93 & 2.08 & 93.15 & 6.24 & 95.80 & 0.19 & 96.27 \\
& Dynamic-all & 100 & 97.05 & 66.31 & 45.46 & 67.73 & 77.42 & 2.49 & 92.89 & 7.03 & 95.62 & 0.26 & 95.94 \\
%  & CLB & 99.83\% & 83.43\% & 54.95\% & 81.53\% & 19.86\% & 77.36\% & 16.11\% & 80.73\% & \textbf{0\%} & \textbf{89.03\%} \\ 
%   & FC & 88.52\% & 83.3& \textbf{29.81\%} & \textbf{84.66\%}
  \cline{2-12}  
   & \multicolumn{1}{l}{Mean ASR Drop} & \multicolumn{1}{|l}{97.73} & \multicolumn{1}{l}{83.55} & \multicolumn{1}{|l}{75.07} & \multicolumn{1}{l}{80.62} & \multicolumn{1}{|l}{24.38} & \multicolumn{1}{l}{76.56} & \multicolumn{1}{|l}{20.40} & \multicolumn{1}{l}{80.37}  & \multicolumn{1}{|c}{\textbf{7.69}} & \multicolumn{1}{c}{\textbf{84.76}} \\ 

 \bottomrule
\end{tabular}
\vspace{-0.1in}
\end{table}

\begin{table}[ht]
    \centering
    \scalebox{0.8}{
    \begin{tabular}{c|cccccc|cccccc}
    \toprule
    Dataset & \multicolumn{6}{c|}{CIFAR10} & \multicolumn{6}{c}{GTSRB} \\
    \midrule
    Method & No Def & {MCR} & {NAD} & {ANP} & ABL & Ours  & No Def & {MCR} & {NAD} & {ANP} & ABL & Ours \\
    \midrule
    None & & & &  & & & &  & & & & \\
    Badnets & & & &  & & & &  & & & &  \\
    Blend & & & &  & & & &  & & & &  \\
    Trojan-one & & & &  & & & &  & & & &  \\
    Trojan-all & & & &  & & & &  & & & &\\
    SIG & & & &  & & & &  & & & &   \\
    Dynamic-one & & & &  & & & &  & & & & \\
    Dynamic-all & & & &  & & & &  & & & &  \\
    CLB & & & &  & & & &  & & & & \\
    % Feature & & & &  & & & &  & & & & \\
    FC & & & &  & & & &  & & & & \\   
    \bottomrule
    \end{tabular}
    }
    \vspace{2mm}
    \caption{Robust Generalization Gap for CIFAR10 and GTSRB. make it multi column for CIFAR10 and GTSRB}
    \label{tab:gtsrb_defense}
\end{table}

\subsubsection{Why some of these techniques fail and others prevail?}
Mostly, we explain why adversarial augmentations comparatively perform poorly than the strong augmentations. We bring in the regularization perspective to explain these results. 

\subsection{Backdoor Removal for Strongly Augmentated Models}
Remove backdoor from the strongly augmented models. See if it gets tougher to remove the backdoor. 

\subsection{Backdoor Removal for Adversarially Trained Models}
**UMAR(***) Remove backdoor from the strongly augmented models. See if it gets tougher to remove.
We have further conducted experiments to eliminate the backdoor attack using five popular augmentation strategies which are: 1) RandAud~\cite{cubuk2020randaugment}, 2) Cutmix~\cite{yun2019cutmix}, 3) Augmix~\cite{hendrycks2019augmix}, 4) Mixup~\cite{zhang2017mixup}, 5) Cutout~\cite{devries2017improved}. The results of which against badnets, SIG and blend are shown in Table \ref{tab:sota_aug}.
\begin{table}[ht]
    \centering
    \scalebox{0.85}{
    \begin{tabular}{c|cc|cc|cc}
    \toprule
    Attacks & \multicolumn{2}{c|}{Badnet} & \multicolumn{2}{c|}{SIG} & \multicolumn{2}{c}{Blend} \\
    \midrule
    Augmentation & ASR & ACC & ASR & ACC & ASR & ACC \\
    \midrule
    RandAug & 35.35 & 61.96 & 0.83 &82.36 & 58.48 &80.72 \\
    CutMix & 2.42&87.95 &1.31 &86.16  &99.58  &93.55  \\
    AugMix & 2.13&92.85 &2.17 &86.56  &100&94.66\\
    Mixup &1.98 &92.22 &1.23 &87.15  &100 &94.21 \\
    Cutout&1.33&92.88&1.34&85.44&100&93.68\\
 
    \bottomrule
    \end{tabular}
    }
    \vspace{2mm}
    \caption{Attack removal with different augmentation techniques }
    \label{tab:sota_aug}
\end{table}

\begin{table}[ht]
    \centering
    \scalebox{0.85}{
    \begin{tabular}{c|cc|cc|cc}
    \toprule
    Attacks & \multicolumn{2}{c|}{Badnet} & \multicolumn{2}{c|}{SIG} & \multicolumn{2}{c}{Blend} \\
    \midrule
    Augmentation & ASR & ACC & ASR & ACC & ASR & ACC \\
    \midrule
    Posterize & 96.1 & 93.84 &100 &87.36 &100 &94.85 \\
    Rotate & 2.9&87.2 &100 &87.16  &100  &89.8  \\
    Solarize & 80.5&85.3 &100 &86.67  &85.7 &85.4\\
    Autocontrast &92.5 &94.1&100 &86.9 &100  &94.71    \\
    Equalize &88.4 &88.63 &100 &87.1  &99.8 &90.1 \\
    Invert & 99.0&66.7 &99.0 & 87.5 &100 &63.7 \\
    Color &99.5 &93.7 &100 &87.48  &99.7 &94.38 \\
    Sharpness &95.7& 93.1& 100&86.9  &100 &94.5 \\
    ShearX & 95.7&93.1 &100 &86.7  &100 &94.5 \\
    Contrast &95.8 &93.5 &100 &87.3  &100 & 94.4\\
    Brightness &97.0 &93.2 &99.0 & 87.6 &100 &94.7 \\   
    ShearY &98.6 & 93.9&99.0 &87.64  &100 &94.75\\
    TranslateY &2.5 &92.98 &100 &86.6    &100 &94.3\\
    TranslateX &3.5 &92.78 &100 &86.78  &100 &94.15\\
    \bottomrule
    \end{tabular}
    }
    \vspace{2mm}
    \caption{Backdoor attack with strong augmentations(One at a time). With a poison rate of 5\%. }
    \label{tab:aug_attack}
\end{table}
\begin{table}[ht]
    \centering
    \scalebox{0.85}{
    \begin{tabular}{c|cc|cc|cc}
    \toprule
    Attacks & \multicolumn{2}{c|}{Badnet} & \multicolumn{2}{c|}{SIG} & \multicolumn{2}{c|}{Blend}  \\
    \midrule
    Augmentation & ASR & ACC & ASR & ACC & ASR & ACC \\
    \midrule
    Posterize & 0.67 & 92.50 &0.89 &86.36 &2.51 &93.10  \\
    Rotate & 1.62&88.66 &0.84 &86.36  &1.78 &90.53 \\
    Solarize & 65.74&89.67 &0.90 &86.58 &47.92&91.44\\
    Autocontrast &21.54&92.15&1.22&86.09&13.39&93.5  \\
    Equalize &26.09&90.14&0.92&86.57&12.15&91.94 \\
    Invert & 41.49&81.10&0.89&86.12&0.89&80.99 \\
    Color &5.04&92.58&1.24&86.59&8.98&93.80   \\
    Sharpness &3.52&92.96&0.73&86.56&9.54&94.12 \\
    ShearX & 11.87&92.0&0.74&87.13&3.58&93.31\\
    Contrast &39.18&92.65&1.07&86.64&10.34&93.19\\
    Brightness&44.99&91.78&0.89&85.78&13.37&92.71  \\   
    ShearY &5.41&92.24&100&94.75&13.59&92.89\\
    TranslateY &2.57&92.98&1.07&86.0&100&86.67\\
    TranslateX &3.54&92.78&100&94.15&100&86.78\\
    \bottomrule
    \end{tabular}
    }
    \vspace{2mm}
    \caption{Backdoor attack removal using augmentation policy with model attacked using strong augmentations as reported in Table \ref{tab:aug_attack}.}
    \label{tab:aug_attack_removal}
\end{table}

\begin{table}[ht]
    \centering
    \scalebox{0.85}{
    \begin{tabular}{c|c|c|c|c|c|c|c}
    \toprule

    Augmentation Severity & 1 & 2&3&4&5&6&7 \\
    %\midrule
    ASR & 36.50&10.85&2.55&2.42&2.35&2.33&2.30\\
   %\midrule
    ACC&93.93&92.92&92.67&92.46&92.43&92.38&92.29 \\
    
    \bottomrule
    \end{tabular}
    }
    \vspace{2mm}
    \caption{Using only rotate and equalize as augmentation to clean the blend backdoored model with different augmentation intensity levels.}
    \label{tab:aug_level}
\end{table}

\begin{table}[ht]
    \centering
    \scalebox{0.85}{
    \begin{tabular}{c|cc}
    \toprule

    Batch Size & ASR & ACC \\
    \midrule
    32 & 0.90 $\pm$ 0.01  & 86.4$\pm$ 0.1 \\
    64 & 0.89$\pm$ 0.01 & 86.3$\pm$0.1 \\
    128 & 0.87$\pm$0.01&86.2$\pm$0.1\\
    256 &0.89$\pm$ 0.01 & 86.6$\pm$ 0.1  \\
    512 & 0.91$\pm$ 0.01& 86.7$\pm$0.1\\
    1024 & 0.93$\pm$ 0.01& 86.8$\pm$ 0.1\\
 
    \bottomrule
    \end{tabular}
    }
    \vspace{2mm}
    \caption{Our proposed defense approach performance against SIG attack with different batch-sizes}
    \label{tab:batch_size}
\end{table}

\begin{table}[ht]
    \centering
    \scalebox{0.85}{
    \begin{tabular}{c|cc}
    \toprule
    learning rate & ASR & ACC \\
    \midrule
    0.001 & 1.2 $\pm$ 0.01  & 87.1$\pm$ 0.1 \\
    0.005 & 0.9$\pm$ 0.01 & 87.2$\pm$0.1 \\
    0.01 & 1.0$\pm$0.01&86.8$\pm$0.1\\
    0.015 &1.1$\pm$ 0.01 & 86.7$\pm$ 0.1  \\
    0.02 & 1.2$\pm$ 0.01& 86.6$\pm$0.1\\

    \bottomrule
    \end{tabular}
    }
    \vspace{2mm}
    \caption{Our proposed defense approach performance against SIG attack with different learning rates}
    \label{tab:learning_rate}
\end{table}

\begin{table}[ht]
    \centering
    \scalebox{0.85}{
    \begin{tabular}{c|cc}
    \toprule

    $\#$ of Iterations & ASR & ACC \\
    \midrule
    600 &0.89 $\pm$ 0.01  & 87.1$\pm$ 0.1 \\
    700 & 0.87$\pm$ 0.01 & 86.6$\pm$0.1 \\
    800 & 0.88$\pm$0.01&87.1$\pm$0.1\\
    900 &0.87$\pm$ 0.01 & 87.1$\pm$ 0.1  \\
    1000 & 0.90$\pm$ 0.01& 87.1$\pm$0.1\\

    \bottomrule
    \end{tabular}
    }

    \vspace{2mm}
    \caption{Our proposed defense approach performance against SIG attack with different number of iterations}
    \label{tab:iterations}
\end{table}

\subsection{Strongly augmented Atacks}
\subsection{Weakly, adversarial, strong}

\begin{proof}
\end{proof}
