# Supplementary material for: Efficient Backdoor Removal Through Natural Gradient Fine-tuning
Source: arXiv:2306.17441 source file (2023-06-30)
Supplement: Supplementary file 2 [file appendix_fisher.tex]

\begin{table}[!htp]

\small
\centering
\caption{The attack success rate (ASR \%) and the clean accuracy (CA \%)  of 4 backdoor defense methods against 10 backdoor attacks including 6 classic backdoor attacks and 4 feature-space attacks. \emph{None} means the training data is completely clean.}
  \label{tab1}
\begin{tabular}{c|c|cc|cc|cc|cc|cc|cc}
\toprule
\multirow{2}{*}{Dataset} & \multirow{2}{*}{Method} & \multicolumn{2}{c|}{\begin{tabular}[c|]{@{}c@{}}No Defense\end{tabular}} & \multicolumn{2}{c|}{MCR} & \multicolumn{2}{c|}{NAD} & \multicolumn{2}{c|}{ANP} &\multicolumn{2}{c|}{ABL}&  \multicolumn{2}{c}{\textbf{Ours}}\\ \cline{3-14} 
 &  & ASR & ACC & ASR & ACC & ASR & ACC & ASR & ACC & ASR & ACC & ASR & ACC\\ \hline
\multirow{8}{*}{CIFAR-10} 
& \emph{None} & 0 & 95.26 & 0 & 90.68 & 0 & 92.34 & 0 & 94.98 & 0 & 93.87 & 0 & 95.10  \\ %\cline{2-12} 
& BadNets &  100 & 90.93 & 3.99 & 81.85 & 4.39 & 85.61 & 2.94 & 84.88  & 3.77 & 87.24 & 1.55 & 89.40 \\
& Blend & 100 & 93.98 & 32.77 & 80.39 & 5.28 & 84.99 & 3.84 & 89.20  & 16.89 & 87.80 & 0.53 & 91.77 \\
& Trojan-one & 100 & 88.63 & 20.55 & 79.83  & 17.61 &  83.66 & 5.73 & 84.94 &  4.21 & 86.72 & 2.93 & 87.20 \\
& Trojan-all & 100 & 90.67 & 22.84 & 80.88  & 18.71 & 83.57 & 5.44 & 85.34  & 4.72 & 86.28 & 2.33 & 87.55 \\
& SIG & 99.75 & 88.64 & 0.91  & 82.44  & 2.17 & 84.77 & 0.39 & 84.63 &  0.28 & 87.20 &  0.07 & 87.65 \\
 & Dynamic-one & 100 & 92.77 & 24.83 & 78.69 & 23.29 & 82.61 & 1.75 & 85.36 & 18.24 & 88.34 & 0.42 & 90.74 \\
 & Dynamic-all & 100 & 92.98 & 26.32 & 77.85 & 22.66 & 81.11 & 2.29 & 84.61  & 16.41 & 87.95 & 0.64& 90.35  \\
  & CLB & 100 & 92.81 & 26.24 & 77.80 & 22.81 & 81.21 & 2.22 & 84.61  & 16.41 & 87.65 & 0.69& 90.29\\  %\\ \cline{2-12} 
  & FC & 87.85 & 84.69 &  40.81 & 81.75 & 53.42 & 83.64 & 3.61 & 82.77 & 1.11 & 82.41 & 1.03 & 83.88 \\\cline{2-12} 
 & \multicolumn{1}{l}{Average Drop} & \multicolumn{1}{|l}{97.83} & \multicolumn{1}{l}{83.55} & \multicolumn{1}{|l}{75.07} & \multicolumn{1}{l}{80.62} & \multicolumn{1}{|l}{24.38} & \multicolumn{1}{l}{76.56} & \multicolumn{1}{|l}{20.40} & \multicolumn{1}{l}{80.37}  & \multicolumn{1}{|c}{\textbf{7.69}} & \multicolumn{1}{c}{\textbf{84.76}} \\ \midrule
\multirow{6}{*}{GTSRB} 
   & \emph{None} & 0 & 97.87 & 0 & 95.49 &  0 & 95.18 &  0 & 96.12 & 0 & 96.41 & 0 & 96.70 \\
   & Badnets & 100 & 97.38 & 1.00 & 93.45 & 0.19 & 89.52 & 0.35 & 93.17 & 0.03 & 96.01 & 0.14 & 96.11 \\
   & Blend & 100 & 95.92 & 6.83 & 92.91 & 8.10 & 89.37 & 4.41 & 93.02 & 24.59 & 93.14 & 3.38 & 93.19  \\
   & Trojan-one & 99.50 & 96.27 & 2.76 & 92.98 & 0.37 & 90.02 & 0.81 & 92.74 & 0.36 & 94.95 & 0.21 &  95.18  \\
  &  Trojan-all & 99.71 & 96.08 & 3.25 & 92.18  & 0.98 & 90.27 & 1.16 & 92.51 & 0.91 & 94.01 & 0.27 & 94.87 \\
  &  SIG & 97.13 & 96.93 & 33.98 & 91.83 & 4.64 & 89.36 & 8.17 & 91.82  & 5.13 & 96.33 & 3.24 & 95.48 \\
  &  Dynamic-one & 100 & 97.27 & 64.82 & 43.91 & 68.71 & 76.93 & 2.08 & 93.15 & 6.24 & 95.80 & 0.19 & 96.27 \\
  &  Dynamic-all & 100 & 97.05 & 66.31 & 45.46 & 67.73 & 77.42 & 2.49 & 92.89 & 7.03 & 95.62 & 0.26 & 95.94 \\
%  & CLB & 99.83\% & 83.43\% & 54.95\% & 81.53\% & 19.86\% & 77.36\% & 16.11\% & 80.73\% & \textbf{0\%} & \textbf{89.03\%} \\ 
%   & FC & 88.52\% & 83.3& \textbf{29.81\%} & \textbf{84.66\%}
  \cline{2-12}  
   & \multicolumn{1}{l}{Average Drop} & \multicolumn{1}{|l}{97.73} & \multicolumn{1}{l}{83.55} & \multicolumn{1}{|l}{75.07} & \multicolumn{1}{l}{80.62} & \multicolumn{1}{|l}{24.38} & \multicolumn{1}{l}{76.56} & \multicolumn{1}{|l}{20.40} & \multicolumn{1}{l}{80.37}  & \multicolumn{1}{|c}{\textbf{7.69}} & \multicolumn{1}{c}{\textbf{84.76}} \\ 

 \bottomrule
\end{tabular}
\vspace{-0.1in}
\end{table}

%%%%%%%%%%%%%%%%%%%%%%%%%%%%%%%%%%%%%%%%%%%%%%%%%%%%%%%%%%%%%%%%%%%

\section{Appendix}

% In this paper, we aim to establish a relationship between the flatness of the weight loss landscape and the backdoor properties of DNN. We hypothesize that backdooring creates unwanted sharp peaks that activates the  (need proof of this). 

% \begin{itemize}
%     \item Using \emph{Extreme Value Analysis}, we first show that the statistics from fisher inforamtion matrix (FIM) can help us differentiate between a backdoor and a benign model.   
%     \item With extensive empirical analysis, we show that FIM based regularization flattens the loss landscape and effectively removes the backdoor. 
%     \item  Furthermore, we theoritically establish that flattening the loss landscape helps cleaning a backdoored model. 
%     \item Our extensive experimental analysis 
% \end{itemize}
{\color{blue} Observations from Table~\ref{tab:CNN-CL-comp}.
\begin{itemize}
    \item CNN backbone is critical to preserve prior learned information of a model. To preserve the clean data accuracy of a backdoored model, intuitively we should keep the parameters of CNN backbone as similar as the original backdoored model.
    \item In case of backdoor insertion, classification layer is the most sensitive layer and highly influenced by poison samples. {\color{red} we will add learning graph to observe the sensitivity of last layer compared with others.}
    \item Takeaway: We will investigate last layer instead of whole network to purify a backdoored model.
\end{itemize}
Analysis: 
\begin{itemize}
    \item First analysis will validate/support our approach towards last layer based purification process. This analysis will be based on Table~\ref{tab:CNN-CL-comp}.
    \item Why do we focus on optimization??! 
    \begin{itemize}
        \item one set of experiments will demonstrate the faster convergence of FIM than SGD's.
        \item Will try to connect the under-parameter analogy
        \item loss landscape will be a metric to show the improvement of generalization of the model over clean data distribution. 
    \end{itemize}
\end{itemize}
}

\begin{itemize}
    \item tiny validation set
    \item need to avoid costly adversarial search problem
    \item use minimal fine-tuning to leverage the catastrophic forgetting properties of NN
    \item problem becomes under-parameterized model if we consider last few layers of DNN
    \item non-convex minimization problem with locally-convex local minima
    \item use NGD with FIM to aviod local minima!
\end{itemize}

Catastrophic forgetting~\cite{kumaran2016learning}

However, as we consider fine-tuning only one layer, the optimization problem can essentially become an under-parameterized non-convex optimization problem. A well-known issue with under-parameterized non-convex optimization is the existence of locally-convex minima~\cite{liu2022loss}. SGD typically fails to get an optimal solution in such optimization problems due to the unawareness of loss curvature knowledge and often provides solutions at local minima. To tackle issues related to local minima, we use loss surface geometry-aware optimization approaches, for instance, second-order optimization algorithms (\eg Natural gradient descent (NGD)~\cite{amari2000adaptive}). From the information geometry perspective, however, NGD defines the update directions in parameter space following the largest change of objective function in per unit change of Kullback-Leibler (KL) divergence between consecutive iterations~\cite{amari2000methods}, in contrast to the Euclidean distance-based SGD and its variants. \textcolor{magenta}{last line is too complicated.}

NGD requires an estimation of the variance of gradient of log-likelihood function, knwon as Fisher Information Matrix (FIM). Due to the parameter space geometry awareness of NDG, we hypothesize that a model purifying step of a trained model using a benign validation data set would remove the backdoor from the model, assuming that the validation data set will include samples from every class in the training data set.

% \section{Appendix}

% Optionally include extra information (complete proofs, additional experiments and plots) in the appendix.
% This section will often be part of the supplemental material.
